# Supplementary material for: Deep Generalized Schr\"odinger Bridge
Source: arXiv:2209.09893 source file (2022-09-20)
Supplement: Supplementary file 1 [file Appendix.pdf]

## A Appendix

### A.1 Summary of Abbreviation and Notation

Table 4: Abbreviation.

|                |                                   |
|----------------|-----------------------------------|
| MFGs           | Mean-Field Games                  |
| SB             | Schrödinger Bridge                |
| DeepRL         | Deep Reinforcement Learning       |
| PDEs           | Partial Differential Equations    |
| HJB            | Hamilton-Jacobi-Bellman           |
| FP             | Fokker-Plank                      |
| SDEs           | Stochastic Differential Equations |
| FBSDEs         | Forward-Backward SDEs             |
| IPF            | Iterative Proportional Fitting    |
| MF interaction | Mean-field interaction            |
| nonlinear FK   | nonlinear Feynman-Kac             |
| TD             | Temporal Difference               |

Table 5: Notation.

|                                |                                         |
|--------------------------------|-----------------------------------------|
| $t$                            | time coordinate                         |
| $s$                            | reversed time coordinate                |
| $u(t, x)$                      | value function                          |
| $\rho(t, x)$                   | marginal distribution                   |
| $\rho_0, \rho_{\text{target}}$ | initial/target distributions            |
| $H$                            | Hamiltonian function                    |
| $F$                            | MF interaction function                 |
| $f$                            | MF base drift                           |
| $\sigma$                       | diffusion scaler                        |
| $(\Psi, \hat{\Psi})$           | solution to SB PDEs                     |
| $(Y, Z)$                       | nonlinear FK of $\Psi$                  |
| $(\hat{Y}, \hat{Z})$           | nonlinear FK of $\hat{\Psi}$            |
| $\text{TD}_s$                  | TD target for $Y_s$                     |
| $\widehat{\text{TD}}_t$        | TD target for $\hat{Y}_t$               |
| $\theta$                       | Parameter of $Y$ (and $Z$ )             |
| $\phi$                         | Parameter of $\hat{Y}$ (and $\hat{Z}$ ) |

### A.2 Review of Nonlinear FK Lemma and SB-FBSDE

**Lemma 4** (Nonlinear Feynman-Kac Lemma [18, 42, 43]). *Let  $v \equiv v(x, t)$  be a function that is twice continuously differentiable in  $x \in \mathbb{R}^d$  and once differentiable in  $t \in [0, T]$ , i.e.,  $v \in C^{2,1}(\mathbb{R}^d, [0, T])$ . Consider the following second-order parabolic PDE,*

$$\frac{\partial v}{\partial t} + \frac{1}{2} \text{Tr}(\nabla^2 v G(x, t) G(x, t)^\top) + \nabla v^\top f(x, t) + h(x, v, G(x, t)^\top \nabla v, t) = 0, \quad v(T, x) = \varphi(x), \quad (19)$$

where  $\nabla^2$  denotes the Hessian operator w.r.t.  $x$  and the functions  $f, G, h$ , and  $\varphi$  satisfy proper regularity conditions. Specifically, (i)  $f, G, h$ , and  $\varphi$  are continuous, (ii)  $f(x, t)$  and  $G(x, t)$  are uniformly Lipschitz in  $x$ , and (iii)  $h(x, y, z, t)$  satisfies quadratic growth condition in  $z$ . Then, (19) exists a unique solution  $v$  such that the following stochastic representation (known as the nonlinear Feynman-Kac transformation) holds:

$$Y_t = v(X_t, t), \quad Z_t = G(X_t, t)^\top \nabla v(X_t, t), \quad (20)$$

where  $(X_t, Y_t, Z_t)$  are the unique adapted solutions to the following FBSDEs:

$$\begin{aligned} dX_t &= f(X_t, t)dt + G(X_t, t)dW_t, \quad X_0 = x_0, \\ dY_t &= -h(X_t, Y_t, Z_t, t)dt + Z_t^\top dW_t, \quad Y_T = \varphi(X_T). \end{aligned} \quad (21)$$

The original deterministic PDE solution  $v(x, t)$  can be recovered by taking conditional expectations:

$$\mathbb{E}[Y_t | X_t = x] = v(x, t), \quad \mathbb{E}[Z_t | X_t = x] = G(x, t)^\top \nabla v(x, t).$$

Lemma 4 establishes an intriguing connection between a certain class of (nonlinear) PDEs in (19) and FBSDEs (21) via the nonlinear FK transformation (20). In this work, we adopt a simpler diffusion  $G(x, t) := \sigma$  as a time-invariant scalar but note that our derivation can be extended to more general cases straightforwardly.

**Viscosity solution.** Lemma 4 can be extended to viscosity solutions when the classical solution does not exist. In which case, we will have  $v(x, t) = \lim_{\epsilon \rightarrow \infty} v^\epsilon(x, t)$  converge uniformly in  $(x, t)$

over a compact set, where  $v^\epsilon(x, t)$  is the classical solution to (19) with  $(f_\epsilon, G_\epsilon, h_\epsilon, \varphi_\epsilon)$  converge uniformly toward  $(f, G, h, \varphi)$  over the compact set; see [18, 55, 56] for a complete discussion.

**SB-FBSDE [27].** Since the PDEs  $(\frac{\partial \Psi}{\partial t}, \frac{\partial \hat{\Psi}}{\partial t})$  appearing in the vanilla SB (4) are both of the parabolic form (19), one can apply Lemma 4 and derive the corresponding nonlinear generators  $h$ . This, as shown in SB-FBSDE [27], leads to the following FBSDEs:

$$\begin{cases} dX_t = (f_t + \sigma Z_t) dt + \sigma dW_t & (22a) \\ dY_t = \frac{1}{2} \|Z_t\|^2 dt + Z_t^\top dW_t & (22b) \\ d\hat{Y}_t = \left( \frac{1}{2} \|\hat{Z}_t\|^2 + \nabla \cdot (\sigma \hat{Z}_t - f_t) + \hat{Z}_t^\top Z_t \right) dt + \hat{Z}_t^\top dW_t & (22c) \end{cases}$$

Further, the nonlinear FK transformation reads

$$\begin{aligned} Y_t &= \log \Psi(X_t, t), & Z_t &= \sigma \nabla \log \Psi(X_t, t), \\ \hat{Y}_t &= \log \hat{\Psi}(X_t, t), & \hat{Z}_t &= \sigma \nabla \log \hat{\Psi}(X_t, t), \end{aligned}$$

which immediately suggests that

$$\mathbb{E}[Y_t | X_t = x] = \log \Psi(x, t), \quad \mathbb{E}[\hat{Y}_t | X_t = x] = \log \hat{\Psi}(x, t). \quad (23)$$

It can be readily seen that (22) is a special case of our Theorem 1 when the MF interaction  $F(x, \rho)$ , which plays a crucial role in MFGs, vanishes. Since SB-FBSDE was primarily developed in the context of generative modeling [57], its training relies on computing the log-likelihood at the boundaries. These log-likelihoods can be obtained by noticing that  $\log \rho(x, t) = \mathbb{E}[Y_t + \hat{Y}_t | X_t = x]$ , as implied by (23) and (8). When  $\hat{Z}_\phi(X_t, t) \approx \hat{Z}_t$  and  $Z_\theta(\bar{X}_s, s) \approx Z_s$ , the training objectives of SB-FBSDE can be computed as the parametrized variational lower-bounds:

$$\log \rho_0(\phi; x) \geq \mathcal{L}_{\text{IPF}}(\phi) := \mathbb{E}[Y_t^\theta + \hat{Y}_t^\phi | X_t = x, t = 0] = \int_t \mathbb{E} [dY_t^\theta + d\hat{Y}_t^\phi | X_0 = x], \quad (24a)$$

$$\log \rho_T(\theta; x) \geq \mathcal{L}_{\text{IPF}}(\theta) := \mathbb{E}[Y_s^\theta + \hat{Y}_s^\phi | \bar{X}_s = x, s = 0] = \int_s \mathbb{E} [dY_s^\theta + d\hat{Y}_s^\phi | \bar{X}_0 = x]. \quad (24b)$$

Invoking (22) to expand the *r.h.s.* of (24) leads to the expression synthesized in (6):

$$\begin{aligned} \mathcal{L}_{\text{IPF}}(\theta) &= \int_0^T \mathbb{E}_{(3b)} \left[ \frac{1}{2} \|Z_\theta(\bar{X}_s, s)\|_2^2 + Z_\theta(\bar{X}_s, s)^\top \hat{Z}_\phi(\bar{X}_s, s) + \nabla \cdot (\sigma Z_\theta(\bar{X}_s, s) + f) \right] ds, \\ \mathcal{L}_{\text{IPF}}(\phi) &= \int_0^T \mathbb{E}_{(3a)} \left[ \frac{1}{2} \|\hat{Z}_\phi(X_t, t)\|_2^2 + \hat{Z}_\phi(X_t, t)^\top Z_\theta(X_t, t) + \nabla \cdot (\sigma \hat{Z}_\phi(X_t, t) - f) \right] dt. \end{aligned}$$

Since (24) concern only the integration over the expectations, *i.e.*,  $\int \mathbb{E}[dY + d\hat{Y}]$ , the solutions  $(Y_t, \hat{Y}_t)$  to the SDEs (22b, 22c) were *never* computed explicitly in SB-FBSDE. This is in contrast to our DeepGSB, which, crucially, requires constructing explicit TD objectives for  $Y$  and  $\hat{Y}$  so that the stochastic dynamics of  $dY$  and  $d\hat{Y}$  are respectively respected. It is clear that the training objectives in (24) are equivalent to (6) up to some independent constant.

### A.3 Proofs in Sec. 3

#### A.3.1 Lemmas

**Relation between  $\mathcal{L}_{\text{IPF}}$  in (6) and KL divergence.** Resemblance between the alternate training of (24), or equivalently (6), and KL divergences was briefly mentioned in [27], yet the formal connection has not yet been established. We provide the following result for completeness and later derivations.

**Lemma 5.** Let  $q^\theta$  and  $q^\phi$  be the marginal densities of the parametrized forward and backward SDEs

$$dX_t^\theta = (f_t + \sigma Z_\theta(X_t^\theta, t)) dt + \sigma dW_t, \quad (25a)$$

$$d\bar{X}_s^\phi = (-f_s + \sigma \hat{Z}_\phi(\bar{X}_s^\phi, t)) ds + \sigma dW_s, \quad (25b)$$

Assuming  $(Z_\theta, q^\theta)$  and  $(\widehat{Z}_\phi, q^\phi)$  satisfy proper regularity (e.g., App. A in [27, 58]) such that

$$\forall t \in [0, T], \exists k > 0 : \quad q_t^\theta(x) = \mathcal{O}(e^{-\|x\|_2^k}) \quad \text{and} \quad q_t^\phi(x) = \mathcal{O}(e^{-\|x\|_2^k})$$

as  $\|x\|_2 \rightarrow \infty$ , then we have

$$D_{\text{KL}}(q^\theta \| q^\phi) = \mathcal{L}_{\text{IPF}}(\phi) + \mathcal{O}(1), \quad \text{and} \quad D_{\text{KL}}(q^\phi \| q^\theta) = \mathcal{L}_{\text{IPF}}(\theta) + \mathcal{O}(1),$$

where  $\mathcal{L}_{\text{IPF}}$  is defined in (6), and  $\mathcal{O}(1)$  is independent of the optimizing variables,  $\phi$  or  $\theta$ .

*Proof.* Recall that the parametrized forward SDE in (25a) can be reversed [57, 59] as

$$dX_s^\theta = (-f_s - \sigma Z_\theta(X_s^\theta, s) + \sigma^2 \nabla \log q^\theta(X_s^\theta, s)) ds + \sigma dW_s,$$

Then, the KL divergence can be expanded by

$$\begin{aligned} & D_{\text{KL}}(q^\theta \| q^\phi) \\ \stackrel{(*)}{=} & \mathbb{E}_{q^\theta} \left[ \int_0^T \frac{1}{2\sigma^2} \|\sigma \widehat{Z}_\phi + \sigma Z_\theta - \sigma^2 \nabla \log q_s^\theta\|^2 ds \right] + D_{\text{KL}}(q_{s=0}^\theta \| \rho_{\text{target}}) \\ = & \int_0^T \mathbb{E}_{q_s^\theta} \left[ \frac{1}{2} \|\widehat{Z}_\phi + Z_\theta\|^2 - \sigma(\widehat{Z}_\phi + Z_\theta)^\top \nabla \log q_s^\theta + \frac{1}{2} \|\sigma \nabla \log q_s^\theta\|^2 \right] ds + D_{\text{KL}}(q_0^\theta \| \rho_{\text{target}}) \\ = & \int_0^T \mathbb{E}_{q_s^\theta} \left[ \frac{1}{2} \|\widehat{Z}_\phi\|^2 + \widehat{Z}_\phi^\top Z_\theta - \sigma \widehat{Z}_\phi^\top \nabla \log q_s^\theta \right] ds \\ & + \underbrace{\int_0^T \mathbb{E}_{q_s^\theta} \left[ \frac{1}{2} \|Z_\theta\|^2 - \sigma Z_\theta^\top \nabla \log q_s^\theta + \frac{1}{2} \|\sigma \nabla \log q_s^\theta\|^2 \right] ds}_{\text{independent of } \phi} + D_{\text{KL}}(q_0^\theta \| \rho_{\text{target}}) \\ = & \int_0^T \mathbb{E}_{q_s^\theta} \left[ \frac{1}{2} \|\widehat{Z}_\phi\|^2 + \widehat{Z}_\phi^\top Z_\theta + \sigma \nabla \cdot \widehat{Z}_\phi \right] ds + \mathcal{O}(1), \end{aligned} \tag{26}$$

where  $(*)$  is due to the Girsanov's Theorem [60] and the last equality follows by

$$\begin{aligned} \mathbb{E}_{q_s^\theta} \left[ -\sigma \widehat{Z}_\phi^\top \nabla \log q_s^\theta \right] &= \int \left( -\sigma \widehat{Z}_\phi^\top \nabla \log q_s^\theta \right) q_s^\theta dx \\ &= \int -\sigma \widehat{Z}_\phi^\top \nabla q_s^\theta dx \\ &\stackrel{(**)}{=} \int \left[ \sigma \nabla \cdot \widehat{Z}_\phi \right] q_s^\theta dx = \mathbb{E}_{q_s^\theta} \left[ \sigma \nabla \cdot \widehat{Z}_\phi \right], \end{aligned}$$

where  $(**)$  is due to **integration by parts** (notice that the boundary terms vanish due to the regularity assumptions on  $q^\theta$  and  $q^\phi$ ). Similar transformations with divergence operations have been adopted in e.g., Song et al. [58] (see their proof of Theorem 1, or their Eq (33)), and Huang et al. [61] (see their Theorem 3 or the derivation in their Appendix A.1). It is clear that (26) is equivalent to  $\mathcal{L}_{\text{IPF}}(\phi)$  up to some constant  $\nabla \cdot f$  independent of  $\phi$ . A similar relation can be derived between  $D_{\text{KL}}(q^\phi \| q^\theta)$  and  $\mathcal{L}_{\text{IPF}}(\theta)$ .  $\square$

**Remark (alternative derivation using FPE).** It is crucial to notice that the aforementioned expression, i.e.,  $D_{\text{KL}}(q^\theta \| q^\phi) \propto \int \mathbb{E}_{q^\theta} [\frac{1}{2} \|\widehat{Z}_\phi + Z_\theta\|^2 + \sigma \nabla \cdot \widehat{Z}_\phi] ds$ , was established upon the backward time coordinate  $s$ . It is possible to derive the same expression using the forward time coordinate  $t$ . For completeness, we provide the derivation below:

**Lemma 6** (Vargas [62], Proposition 1, Sec 6.3.1).

$$d \log q_t^\phi = \left[ \nabla \cdot (\sigma \widehat{Z}_\phi - f_t) + \sigma (Z_\theta + \widehat{Z}_\phi)^\top \nabla \log q_t^\phi - \frac{1}{2} \|\sigma \nabla \log q_t^\phi\|^2 \right] dt + \sigma \nabla \log q_t^\phi^\top dW_t.$$

*Proof.* Invoking Ito lemma w.r.t. the parameterized forward SDE (25a),

$$d \log q_t^\phi = \left[ \frac{\partial \log q_t^\phi}{\partial t} + \nabla \log q_t^\phi^\top (f_t + \sigma Z_\theta) + \frac{\sigma^2}{2} \Delta \log q_t^\phi \right] dt + \sigma \nabla \log q_t^\phi^\top dW_t,$$

where  $\frac{\partial \log q_t^\phi}{\partial t}$  obeys (see Eq 13.4 in Nelson [63]):

$$\begin{aligned} -\frac{\partial q_t^\phi}{\partial t} &= -\nabla \cdot \left( (\sigma \widehat{Z}_\phi - f_t) q_t^\phi \right) + \frac{\sigma^2}{2} \Delta q_t^\phi \\ \Rightarrow \frac{\partial \log q_t^\phi}{\partial t} &= \nabla \cdot (\sigma \widehat{Z}_\phi - f_t) + (\sigma \widehat{Z}_\phi - f_t)^\top \nabla \log q_t^\phi - \frac{\sigma^2 \Delta q_t^\phi}{2 q_t^\phi}. \end{aligned}$$

Substituting the above relation yields the desired results.  $\square$

**Proposition 7** (Vargas [62], Proposition 1 in Sec 6.3.1).

$$\begin{aligned} D_{\text{KL}}(q^\theta || q^\phi) &= \int_0^T \mathbb{E}_{q_t^\theta} \left[ \frac{1}{2} \|\widehat{Z}_\phi + Z_\theta\|^2 + \nabla \cdot (\sigma \widehat{Z}_\phi - f_t) \right] dt + \mathbb{E}_{q^\theta} \left[ \log \frac{\rho_0}{\rho_{\text{target}}} \right] \\ &\propto \int_0^T \mathbb{E}_{q_t^\theta} \left[ \frac{1}{2} \|\widehat{Z}_\phi + Z_\theta\|^2 + \sigma \nabla \cdot \widehat{Z}_\phi \right] dt + \mathcal{O}(1), \end{aligned}$$

where  $\mathcal{O}(1)$  collects all terms independent of  $\phi$ .

*Proof.* The proof essentially follows Vargas [62] by adopting our notations. Recall that the parametrized backward SDE (25b) can be reversed [57, 59] as

$$d\bar{X}_t^\phi = \left( f_t - \sigma Z_\theta(\bar{X}_t^\phi, t) + \sigma^2 \nabla \log q^\phi(\bar{X}_t^\phi, t) \right) dt + \sigma dW_t.$$

Then, we have

$$\begin{aligned} D_{\text{KL}}(q^\theta || q^\phi) &= \int_0^T \mathbb{E}_{q_t^\theta} \left[ \frac{1}{2} \|\widehat{Z}_\phi + Z_\theta - \sigma \nabla \log q_t^\phi\|^2 \right] dt + D_{\text{KL}}(\rho_0 || q_{t=0}^\phi) \\ &= \int_0^T \mathbb{E}_{q_t^\theta} \left[ \frac{1}{2} \|\widehat{Z}_\phi + Z_\theta\|^2 - \sigma (\widehat{Z}_\phi + Z_\theta)^\top \nabla \log q_t^\phi + \frac{1}{2} \|\sigma \nabla \log q_t^\phi\|^2 \right] dt + D_{\text{KL}}(\rho_0 || q_{t=0}^\phi) \\ &\stackrel{(*)}{=} \int_0^T \mathbb{E}_{q_t^\theta} \left[ \frac{1}{2} \|\widehat{Z}_\phi + Z_\theta\|^2 + \nabla \cdot (\sigma \widehat{Z}_\phi - f_t) \right] dt - \mathbb{E}_{q^\theta} \left[ \int_0^T d \log q_t^\phi \right] + D_{\text{KL}}(\rho_0 || q_{t=0}^\phi) \\ &= \int_0^T \mathbb{E}_{q_t^\theta} \left[ \frac{1}{2} \|\widehat{Z}_\phi + Z_\theta\|^2 + \nabla \cdot (\sigma \widehat{Z}_\phi - f_t) \right] dt + \mathbb{E}_{q^\theta} \left[ \log \frac{\rho_0}{\rho_{\text{target}}} \right], \end{aligned}$$

where  $(*)$  is due to Lemma 6.  $\square$

**Lemma 8** (Itô formula [44]). *Let  $X_t$  be the solution to the Itô SDE:*

$$dX_t = f(X_t, t)dt + \sigma(X_t, t)dW_t.$$

*Then, the stochastic process  $v(X_t, t)$ , where  $v \in C^{2,1}(\mathbb{R}^d, [0, T])$ , is also an Itô process satisfying*

$$dv(X_t, t) = \frac{\partial v(X_t, t)}{\partial t} dt + \left[ \nabla v(X_t, t)^\top f + \frac{1}{2} \text{Tr} [\sigma^\top \nabla^2 v(X_t, t) \sigma] \right] dt + [\nabla v(X_t, t)^\top \sigma] dW_t. \quad (27)$$

**Lemma 9.** *The following equality holds at any point  $x \in \mathbb{R}^n$  such that  $p(x) \neq 0$ .*

$$\frac{1}{p(x)} \Delta p(x) = \|\nabla \log p(x)\|^2 + \Delta \log p(x)$$

*Proof.*

$$\begin{aligned} \frac{1}{p(x)} \Delta p(x) &= \frac{1}{p(x)} \nabla \cdot \nabla p(x) \\ &= \frac{1}{p(x)} \nabla \cdot (p(x) \nabla \log p(x)) \\ &= \frac{1}{p(x)} (\nabla p(x)^\top \nabla \log p(x) + p(x) \Delta \log p(x)) \\ &= \|\nabla \log p(x)\|^2 + \Delta \log p(x) \end{aligned}$$

$\square$

### A.3.2 Proof of Theorem 1

Now, we begin the proof. Apply the Itô formula to  $v := \log \Psi(X_t, t)$ , where  $X_t$  follows (3a),

$$d \log \Psi = \frac{\partial \log \Psi}{\partial t} dt + \left[ \nabla \log \Psi^\top (f + \sigma^2 \nabla \log \Psi) + \frac{\sigma^2}{2} \Delta \log \Psi \right] dt + \sigma \nabla \log \Psi^\top dW_t,$$

and notice that the PDE of  $\frac{\partial \log \Psi}{\partial t}$  obeys

$$\frac{\partial \log \Psi}{\partial t} = \frac{1}{\Psi} \left( -\nabla \Psi^\top f - \frac{\sigma^2}{2} \Delta \Psi + F \Psi \right) = -\nabla \log \Psi^\top f - \frac{\sigma^2}{2} \|\nabla \log \Psi\|^2 - \frac{\sigma^2}{2} \Delta \log \Psi + F.$$

This yields

$$d \log \Psi = \left[ \frac{1}{2} \|\sigma \nabla \log \Psi\|^2 + F \right] dt + \sigma \nabla \log \Psi^\top dW_t. \quad (28)$$

Now, apply the same Itô formula by instead substituting  $v := \log \hat{\Psi}(X_t, t)$ , where  $X_t$  follows (3a),

$$d \log \hat{\Psi} = \frac{\partial \log \hat{\Psi}}{\partial t} dt + \left[ \nabla \log \hat{\Psi}^\top (f + \sigma^2 \nabla \log \Psi) + \frac{\sigma^2}{2} \Delta \log \hat{\Psi} \right] dt + \sigma \nabla \log \hat{\Psi}^\top dW_t,$$

and notice that the PDE of  $\frac{\partial \log \hat{\Psi}}{\partial t}$  obeys

$$\begin{aligned} \frac{\partial \log \hat{\Psi}}{\partial t} &= \frac{1}{\hat{\Psi}} \left( -\nabla \cdot (\hat{\Psi} f) + \frac{\sigma^2}{2} \Delta \hat{\Psi} - F \hat{\Psi} \right) \\ &= -\nabla \log \hat{\Psi}^\top f - \nabla \cdot f + \frac{\sigma^2}{2} \|\nabla \log \hat{\Psi}\|^2 + \frac{\sigma^2}{2} \Delta \log \hat{\Psi} - F. \end{aligned}$$

This yields

$$\begin{aligned} d \log \hat{\Psi} &= \left[ -\nabla \cdot f + \frac{\sigma^2}{2} \|\nabla \log \hat{\Psi}\|^2 + \sigma^2 \nabla \log \hat{\Psi}^\top \nabla \log \Psi + \sigma^2 \Delta \log \hat{\Psi} - F \right] dt + \sigma \nabla \log \hat{\Psi}^\top dW_t \\ &= \left[ \nabla \cdot (\sigma^2 \nabla \log \hat{\Psi} - f) + \frac{\sigma^2}{2} \|\nabla \log \hat{\Psi}\|^2 + \sigma^2 \nabla \log \hat{\Psi}^\top \nabla \log \Psi - F \right] dt + \sigma \nabla \log \hat{\Psi}^\top dW_t. \end{aligned} \quad (29)$$

Finally, with the nonlinear FK transformation in (10), *i.e.*,

$$\begin{aligned} Y_t &\equiv Y(X_t, t) = \log \Psi(X_t, t), & Z_t &\equiv Z(X_t, t) = \sigma \nabla \log \Psi(X_t, t), \\ \hat{Y}_t &\equiv \hat{Y}(X_t, t) = \log \hat{\Psi}(X_t, t), & \hat{Z}_t &\equiv \hat{Z}(X_t, t) = \sigma \nabla \log \hat{\Psi}(X_t, t), \end{aligned}$$

we can rewrite (3a, 28, 29) as the FBSDEs system in (11).

$$\begin{aligned} dX_t &= (f_t + \sigma Z_t) dt + \sigma dW_t \\ dY_t &= \left[ \frac{1}{2} \|Z_t\|^2 + F_t \right] dt + Z_t^\top dW_t \\ d\hat{Y}_t &= \left[ \frac{1}{2} \|\hat{Z}_t\|^2 + \hat{Z}_t^\top Z_t + \nabla \cdot (\sigma \hat{Z}_t - f_t) - F_t \right] dt + \hat{Z}_t^\top dW_t \end{aligned}$$

where

$$f_t := f(X_t, \exp(Y_t + \hat{Y}_t)), \quad F_t := F(X_t, \exp(Y_t + \hat{Y}_t)).$$

Derivation of the second FBSDEs system in (12) follows a similar flow, except that we need to rebase the PDEs (9) to the “*reversed*” time coordinate  $s := T - t$ . This can be done by reformulating the HJB and FP PDEs in (7) under the  $s$  coordinate, then applying the following Hopf-Cole transform:

$$\hat{\Psi}(x, s) := \exp(-u(x, s)), \quad \Psi(x, s) := \rho(x, s) \exp(u(x, s)). \quad (31)$$

Notice that we flip the role of  $\widehat{\Psi}(x, s)$  and  $\Psi(x, s)$  as the former now relates to the policy appearing in (3b). Omitting the computation similar to Appendix A.4.1, we arrive at the following:

$$\begin{cases} \frac{\partial \widehat{\Psi}(x, s)}{\partial s} = \nabla \widehat{\Psi}^\top f - \frac{1}{2} \sigma^2 \Delta \widehat{\Psi} + F \widehat{\Psi} \\ \frac{\partial \Psi(x, s)}{\partial s} = \nabla \cdot (\Psi f) + \frac{1}{2} \sigma^2 \Delta \Psi - F \Psi \end{cases} \quad \text{s.t.} \quad \begin{cases} \widehat{\Psi}(\cdot, 0) \Psi(\cdot, 0) = \rho_{\text{target}} \\ \widehat{\Psi}(\cdot, T) \Psi(\cdot, T) = \rho_0 \end{cases}. \quad (32)$$

Apply the Itô formula to  $v := \log \Psi(\bar{X}_s, s)$ , where  $\bar{X}_s$  evolves along the reversed SDE (3b).

$$d \log \Psi = \frac{\partial \log \Psi}{\partial s} ds + \left[ \nabla \log \Psi^\top (-f + \sigma^2 \nabla \log \widehat{\Psi}) + \frac{\sigma^2}{2} \Delta \log \Psi \right] ds + \sigma \nabla \log \Psi^\top dW_s,$$

and notice that the PDE of  $\frac{\partial \log \Psi}{\partial s}$  now obeys

$$\begin{aligned} \frac{\partial \log \Psi}{\partial s} &= \frac{1}{\Psi} \left( \nabla \cdot (\Psi f) + \frac{\sigma^2}{2} \Delta \Psi - F \Psi \right) \\ &= \nabla \log \Psi^\top f + \nabla \cdot f + \frac{\sigma^2}{2} \|\nabla \log \Psi\|^2 + \frac{\sigma^2}{2} \Delta \log \Psi - F. \end{aligned}$$

This yields

$$\begin{aligned} d \log \Psi &= \left[ \nabla \cdot f + \frac{\sigma^2}{2} \|\nabla \log \Psi\|^2 + \sigma^2 \nabla \log \Psi^\top \nabla \log \widehat{\Psi} + \sigma^2 \Delta \log \Psi - F \right] ds + \sigma \nabla \log \Psi^\top dW_s \\ &= \left[ \nabla \cdot (f + \sigma^2 \nabla \log \Psi) + \frac{\sigma^2}{2} \|\nabla \log \Psi\|^2 + \sigma^2 \nabla \log \Psi^\top \nabla \log \widehat{\Psi} - F \right] ds + \sigma \nabla \log \Psi^\top dW_s. \end{aligned} \quad (33)$$

Similarly, apply the Itô formula to  $v := \log \widehat{\Psi}(\bar{X}_s, s)$ , where  $\bar{X}_s$  follows the same reversed SDE (3b).

$$d \log \widehat{\Psi} = \frac{\partial \log \widehat{\Psi}}{\partial s} ds + \left[ \nabla \log \widehat{\Psi}^\top (-f + \sigma^2 \nabla \log \widehat{\Psi}) + \frac{\sigma^2}{2} \Delta \log \widehat{\Psi} \right] ds + \sigma \nabla \log \widehat{\Psi}^\top dW_s,$$

and notice that the PDE of  $\frac{\partial \log \widehat{\Psi}}{\partial s}$  obeys

$$\frac{\partial \log \widehat{\Psi}}{\partial s} = \frac{1}{\widehat{\Psi}} \left( \nabla \widehat{\Psi}^\top f - \frac{\sigma^2}{2} \Delta \widehat{\Psi} + F \widehat{\Psi} \right) = \nabla \log \widehat{\Psi}^\top f - \frac{\sigma^2}{2} \|\nabla \log \widehat{\Psi}\|^2 - \frac{\sigma^2}{2} \Delta \log \widehat{\Psi} + F.$$

This yields

$$d \log \widehat{\Psi} = \left[ \frac{1}{2} \|\sigma \nabla \log \widehat{\Psi}\|^2 + F \right] ds + \sigma \nabla \log \widehat{\Psi}^\top dW_s. \quad (34)$$

Finally, with a nonlinear FK transformation similar to (10),

$$\begin{aligned} Y_s &\equiv Y(\bar{X}_s, s) = \log \Psi(\bar{X}_s, s), & Z_s &\equiv Z(\bar{X}_s, s) = \sigma \nabla \log \Psi(\bar{X}_s, s), \\ \widehat{Y}_s &\equiv \widehat{Y}(\bar{X}_s, s) = \log \widehat{\Psi}(\bar{X}_s, s), & \widehat{Z}_s &\equiv \widehat{Z}(\bar{X}_s, s) = \sigma \nabla \log \widehat{\Psi}(\bar{X}_s, s), \end{aligned} \quad (35)$$

we can rewrite (3b, 33, 34) as the second FBSDEs system in (12).

$$\begin{aligned} d\bar{X}_s &= (-f_s + \sigma \widehat{Z}_s) ds + \sigma dW_s \\ dY_s &= \left( \frac{1}{2} \|Z_s\|^2 + \nabla \cdot (\sigma Z_s + f_s) + Z_s^\top \widehat{Z}_s - F_s \right) ds + Z_s^\top dW_s \\ d\widehat{Y}_s &= \left( \frac{1}{2} \|\widehat{Z}_s\|^2 + F_s \right) ds + \widehat{Z}_s^\top dW_s \end{aligned}$$

where

$$f_s := f(\bar{X}_s, \exp(Y_s + \widehat{Y}_s)), \quad F_s := F(\bar{X}_s, \exp(Y_s + \widehat{Y}_s)).$$

We conclude the proof.  $\square$

### A.3.3 Proof of Proposition 2

*Proof.* We will only prove the TD objective (14a) for the time coordinate  $t$ , as all derivations can be adopted similarly to its reversed coordinate  $s := T - t$ .

Given a realization of the parametrized SDE (11a) w.r.t. some fixed step size  $\delta t$ , i.e.,

$$X_{t+\delta t}^\theta = X_t^\theta + (f_t + \sigma Z_\theta(X_t^\theta, t)) \delta t + \delta W_t, \quad \delta W_t \sim \mathcal{N}(\mathbf{0}, \delta t \mathbf{I}),$$

we can represent the trajectory compactly by a sequence of tuples  $\mathbf{X}_k^\theta \equiv (X_k^\theta, Z_k^\theta, \delta W_k)$  sampled on some discrete time grids,  $k \in \{0, \dots, t, t + \delta t, \dots, T\}$ . The incremental change of  $\hat{Y}_t$ , i.e., the r.h.s. of (11c), can then be computed by

$$\delta \hat{Y}_t(\mathbf{X}_t^\theta) := \left( \frac{1}{2} \|\hat{Z}(X_t^\theta, t)\|^2 + \nabla \cdot (\sigma \hat{Z}(X_t^\theta, t) - f_t) + \hat{Z}(X_t^\theta, t)^\top Z_t^\theta - F_t \right) \delta t + \hat{Z}(X_t^\theta, t)^\top \delta W_t,$$

where  $\hat{Z}(\cdot, \cdot)$  is the (parametrized) backward policy and we denote  $Z_t^\theta := Z_\theta(X_t^\theta, t)$  for simplicity. At the equilibrium when the FBSDE system (11) is satisfied, the SDE (11c) must hold. This suggests the following equality:

$$\hat{Y}(X_{t+\delta t}^\theta, t + \delta t) = \hat{Y}(X_t^\theta, t) + \delta \hat{Y}_t(\mathbf{X}_t^\theta). \quad (37)$$

Hence, we can interpret the r.h.s. of (37) as the single-step TD target  $\widehat{\text{TD}}_{t+\delta t}^{\text{single}}$ , which yields the expression in (14a). The multi-step TD target can be constructed accordingly as standard practices [49, 50], and either TD target can be used to construct the TD objective for the parametrized function  $\hat{Y}_\phi \approx \hat{Y}$ , which further yields (16).  $\square$

### A.3.4 Proof of Proposition 3

*Proof.* We first prove the necessary condition. Suppose the parametrized functions  $(Y_\theta, Z_\theta, \hat{Y}_\phi, \hat{Z}_\phi)$  satisfy the SDEs in (11, 12), it can be readily seen that the TD objectives  $\mathcal{L}_{\text{TD}}(\phi)$  and  $\mathcal{L}_{\text{TD}}(\theta)$  shall both be minimized, as the parametrized functions satisfy (11c, 12b). Next, notice that (11) implies

$$\begin{aligned} Y_T^\theta + \hat{Y}_T^\phi &= \left( Y_0^\theta + \int_0^T dY_t^\theta \right) + \left( \hat{Y}_0^\phi + \int_0^T d\hat{Y}_t^\phi \right) \\ \Rightarrow 0 &= \mathbb{E}_{q^\theta} \left[ \left( Y_0^\theta + \hat{Y}_0^\phi \right) + \int_0^T \left( dY_t^\theta + d\hat{Y}_t^\phi \right) - \left( Y_T^\theta + \hat{Y}_T^\phi \right) \right] \\ &\stackrel{(*)}{=} \mathbb{E}_{q_0^\theta} [\log \rho_0] + \int_0^T \mathbb{E}_{q_t^\theta} \left[ \frac{1}{2} \|Z_t^\theta + \hat{Z}_t^\phi\|^2 + \nabla \cdot (\sigma \hat{Z}_t^\phi - f_t) \right] dt - \mathbb{E}_{q_T^\theta} [\log \rho_{\text{target}}] \\ &\stackrel{(**)}{=} \mathbb{E}_{q_0^\theta} [\log \rho_0] + D_{\text{KL}}(q^\theta \| q^\phi) - \mathbb{E}_{q^\theta} \left[ \log \frac{\rho_0}{\rho_{\text{target}}} \right] - \mathbb{E}_{q_T^\theta} [\log \rho_{\text{target}}] \\ &= D_{\text{KL}}(q^\theta \| q^\phi), \end{aligned}$$

where (\*) is due to (11b, 11c) and (\*\*) invokes Proposition 7. The fact that  $\mathcal{L}_{\text{IPF}}(\phi) \propto D_{\text{KL}}(q^\theta \| q^\phi) = 0$  (recall Lemma 5) suggests that the objective  $\mathcal{L}_{\text{IPF}}(\phi)$  is minimized when (11) holds. Finally, as similar arguments can be adopted to  $\mathcal{L}_{\text{IPF}}(\theta) \propto D_{\text{KL}}(q^\phi \| q^\theta) = 0$  when (12) holds, we conclude that all losses are minimized when the parameterized functions satisfy the FBSDE systems (11, 12).

We proceed to proving the sufficient condition, which is more involved. First, notice that

$$\mathcal{L}_{\text{IPF}}(\phi) \text{ is minimized} \Leftrightarrow D_{\text{KL}}(q^\theta \| q^\phi) = 0 \Leftrightarrow \forall s \in [0, T], \quad Z_s^\theta + \hat{Z}_s^\phi - \sigma \nabla \log q_s^\theta = 0, \quad (38)$$

$$\mathcal{L}_{\text{IPF}}(\theta) \text{ is minimized} \Leftrightarrow D_{\text{KL}}(q^\phi \| q^\theta) = 0 \Leftrightarrow \forall t \in [0, T], \quad Z_t^\theta + \hat{Z}_t^\phi - \sigma \nabla \log q_t^\phi = 0, \quad (39)$$

as implied by (26). If  $\mathcal{L}_{\text{TD}}(\phi)$  and  $\mathcal{L}_{\text{TD}}(\theta)$  are minimized, the following relations must also hold

$$d\hat{Y}_t^\phi = \left( \frac{1}{2} \|\hat{Z}_t^\phi\|^2 + \nabla \cdot (\sigma \hat{Z}_t^\phi - f_t) + Z_t^{\theta^\top} \hat{Z}_t^\phi - F_t \right) dt + \hat{Z}_t^{\phi^\top} dW_t, \quad (40)$$

$$dY_s^\theta = \left( \frac{1}{2} \|Z_s^\theta\|^2 + \nabla \cdot (\sigma \hat{Z}_s^\phi + f_s) + Z_s^{\theta^\top} \hat{Z}_s^\phi - F_s \right) dt + Z_s^{\theta^\top} dW_s. \quad (41)$$

Now, recall the parametrized forward SDE:

$$dX_t^\theta = (f_t + \sigma Z_\theta(X_t^\theta, t)) dt + \sigma dW_t, \quad (42)$$

whose Fokker Plank equation obeys

$$\frac{\partial q_t^\theta}{\partial t} = -\nabla \cdot (q_t^\theta (f_t + \sigma Z_t^\theta)) + \frac{1}{2} \sigma^2 \Delta q_t^\theta,$$

which implies that (c.f. Lemma 9),

$$\frac{\partial \log q_t^\theta}{\partial t} = -\nabla \cdot (f_t + \sigma Z_t^\theta) - \nabla \log q_t^{\theta^\top} (f_t + \sigma Z_t^\theta) + \frac{\sigma^2}{2} (\Delta \log q_t^\theta + \|\nabla \log q_t^\theta\|^2).$$

Invoking Ito lemma and substituting the above PDE yield:

$$\begin{aligned} d \log q_t^\theta &= \frac{\partial \log q_t^\theta}{\partial t} dt + \left[ \nabla \log q_t^{\theta^\top} (f_t + \sigma Z_t^\theta) + \frac{\sigma^2}{2} \Delta \log q_t^\theta \right] dt + \sigma \nabla \log q_t^{\theta^\top} dW_t \\ &= \left[ -\nabla \cdot (f_t + \sigma Z_t^\theta) + \sigma^2 \Delta \log q_t^\theta + \frac{\sigma^2}{2} \|\nabla \log q_t^\theta\|^2 \right] dt + \sigma \nabla \log q_t^{\theta^\top} dW_t \\ &= \left[ -\nabla \cdot (f_t + \sigma Z_t^\theta - \sigma^2 \nabla \log q_t^\theta) + \frac{1}{2} \|\sigma \nabla \log q_t^\theta\|^2 \right] dt + \sigma \nabla \log q_t^{\theta^\top} dW_t \\ &\stackrel{(*)}{=} \left[ -\nabla \cdot (f_t + \sigma Z_t^\theta - \sigma (Z_t^\theta + \widehat{Z}_t^\phi)) + \frac{1}{2} \|Z_t^\theta + \widehat{Z}_t^\phi\|^2 \right] dt + (Z_t^\theta + \widehat{Z}_t^\phi)^\top dW_t \\ &= \left[ \nabla \cdot (\sigma \widehat{Z}_t^\phi - f_t) + \frac{1}{2} \|Z_t^\theta + \widehat{Z}_t^\phi\|^2 \right] dt + (Z_t^\theta + \widehat{Z}_t^\phi)^\top dW_t, \end{aligned} \quad (43)$$

where  $(*)$  is due to (38). Subtracting (40) from (43) yields

$$d \log q_t^\theta - d \widehat{Y}_t^\phi = \left( \frac{1}{2} \|Z_t^\theta\|^2 + F_t \right) dt + Z_t^{\theta^\top} dW_t. \quad (44)$$

Now, using the fact that  $Z_\theta := \sigma \nabla Y_\theta$  and  $\widehat{Z}_\phi := \sigma \nabla \widehat{Y}_\phi$ , we know that

$$Z_t^\theta + \widehat{Z}_t^\phi - \sigma \nabla \log q_t^\theta = 0 \Rightarrow Y_t^\theta + \widehat{Y}_t^\phi = \log q_t^\theta + c_t,$$

for some function  $c_t \equiv c(t)$ . Hence, (44) becomes

$$dY_t^\theta - dc_t = \left( \frac{1}{2} \|Z_t^\theta\|^2 + F_t \right) dt + Z_t^{\theta^\top} dW_t. \quad (45)$$

Now we prove that  $\forall t \in (0, T), dc_t = 0$  by contradiction. First, notice that  $c_t$  can be derived analytically as

$$\begin{aligned} c_t &= Y_t^\theta + \widehat{Y}_t^\phi - \log q_t^\theta \\ &= \int_0^t (dY_\tau^\theta + d\widehat{Y}_\tau^\phi - d \log q_\tau^\theta) \\ &\stackrel{(*)}{=} \int_0^t \left( \left( \frac{\partial Y_\tau^\theta}{\partial \tau} + \nabla Y_\tau^{\theta^\top} (f_\tau + \sigma Z_\tau^\theta) + \frac{\sigma^2}{2} \Delta Y_\tau^\theta \right) - \left( \frac{1}{2} \|Z_\tau^\theta\|^2 + F_\tau \right) \right) d\tau \\ &\quad + \int_0^t (\sigma \nabla Y_\tau^{\theta^\top} dW_\tau - Z_\tau^{\theta^\top} dW_\tau) \\ &\stackrel{(**)}{=} \int_0^t \left( \frac{\partial Y_\tau^\theta}{\partial t} - \left( -\nabla Y_\tau^{\theta^\top} f_\tau - \frac{1}{2} \|\sigma \nabla Y_\tau^\theta\|^2 - \frac{\sigma^2}{2} \Delta Y_\tau^\theta + F_\tau \right) \right) d\tau, \end{aligned} \quad (46)$$

where  $(*)$  invokes the following Ito lemma and substitutes (44),

$$dY_\tau^\theta = \frac{\partial Y_\tau^\theta}{\partial \tau} d\tau + \left[ \nabla Y_\tau^{\theta^\top} (f_\tau + \sigma Z_\tau^\theta) + \frac{\sigma^2}{2} \Delta Y_\tau^\theta \right] dt + \sigma \nabla Y_\tau^{\theta^\top} dW_\tau,$$

and  $(**)$  substitutes the definition  $Z_\tau^\theta := \sigma \nabla Y_\tau^\theta$ . Equation (46) has an intriguing implication, as one can verify that its integrand is the *residual of the parametrized HJB*  $Y_\theta = -u_\theta \approx -u$  (recall (7) and



(8)). It is straightforward to see that, the residual shall also be preserved after the parametrized HJB is expanded by Ito lemma w.r.t. the backward parametrized SDE:

$$d\bar{X}_s^\phi = \left(-f_s + \sigma \hat{Z}_\phi(\bar{X}_s^\phi, s)\right) ds + \sigma dW_s. \quad (47)$$

That is, the following equation similar to (45) must hold for some function  $c_s := c(T - t)$ :

$$dY_s^\theta + dc_s = \left(\frac{1}{2}\|Z_s^\theta\|^2 + \nabla \cdot (f_s + \sigma \hat{Z}_s^\phi) + Z_s^{\theta^\top} \hat{Z}_s^\phi - F_s\right) dt + Z_s^{\theta^\top} dW_s,$$

which contradicts (41). Hence, we must have  $dc_s = dc_t = 0$ , and (45) becomes

$$dY_t^\theta = \left(\frac{1}{2}\|Z_t^\theta\|^2 + F_t\right) dt + Z_t^{\theta^\top} dW_t. \quad (48)$$

In short, we have shown that, for the parametrized forward (42) and backward (47) SDEs, the fact that (40, 41) hold implies that (48) holds, providing  $\mathcal{L}_{\text{IPF}}(\phi)$  is minimized. The exact same statement can be repeated to prove that

$$d\hat{Y}_s^\phi = \left(\frac{1}{2}\|\hat{Z}_s^\phi\|^2 + F_s\right) ds + \hat{Z}_s^{\phi^\top} dW_s. \quad (49)$$

Therefore, if the combined objectives are minimized, *i.e.*, (38, 39, 40, 41) hold, the parametrized functions  $(Y_\theta, Z_\theta, \hat{Y}_\phi, \hat{Z}_\phi)$  satisfy (42, 40, 48, 47, 41, 49), *i.e.*, they satisfy the FBSDE systems (11, 12) in Theorem 1.  $\square$

#### A.4 Missing Derivations in Sec. 3 and 4

##### A.4.1 Hopf-Cole transform

Recall the Hopf-Cole transform

$$\Psi(x, t) := \exp(-u(x, t)), \quad \hat{\Psi}(x, t) := \rho(x, t) \exp(u(x, t)).$$

Standard ordinary calculus yields

$$\nabla \Psi = -\exp(-u) \nabla u, \quad \Delta \Psi = \exp(-u) [\|\nabla u\|^2 - \Delta u], \quad (50)$$

$$\nabla \hat{\Psi} = \exp(u) (\rho \nabla u + \nabla \rho), \quad \Delta \hat{\Psi} = \exp(u) [\rho \|\nabla u\|^2 + 2 \nabla \rho^\top \nabla u + \Delta \rho + \rho \Delta u]. \quad (51)$$

Hence, we have

$$\begin{aligned} \frac{\partial \Psi}{\partial t} &= \exp(-u) \left(-\frac{\partial u}{\partial t}\right) \\ &\stackrel{(7)}{=} \exp(-u) \left(-\frac{1}{2}\|\sigma \nabla u\|^2 + \nabla u^\top f + \frac{1}{2}\sigma^2 \Delta u + F\right) \\ &\stackrel{(50)}{=} -\frac{1}{2}\sigma^2 \Delta \Psi - \nabla \Psi^\top f + F \Psi, \end{aligned} \quad (52)$$

$$\begin{aligned} \frac{\partial \hat{\Psi}}{\partial t} &= \exp(u) \left(\frac{\partial \rho}{\partial t} + \rho \frac{\partial u}{\partial t}\right) \\ &\stackrel{(7)}{=} \exp(u) \left(\left(\nabla \cdot (\rho(\sigma^2 \nabla u - f)) + \frac{1}{2}\sigma^2 \Delta \rho\right) + \rho \left(\frac{1}{2}\|\sigma \nabla u\|^2 - \nabla u^\top f - \frac{1}{2}\sigma^2 \Delta u - F\right)\right) \\ &= \exp(u) \left(\sigma^2 \left(\rho \Delta u + \nabla \rho^\top \nabla u + \frac{1}{2}\Delta \rho + \frac{\rho}{2}\|\nabla u\|^2 - \frac{\rho}{2}\Delta u\right) - \nabla \rho^\top f - \rho \nabla \cdot f - \rho \nabla u^\top f - \rho F\right) \\ &\stackrel{(51)}{=} \frac{1}{2}\sigma^2 \Delta \hat{\Psi} - \nabla \hat{\Psi}^\top f - \hat{\Psi} \nabla \cdot f - \hat{\Psi} F, \end{aligned} \quad (53)$$

which yields (9) by noticing that  $\nabla \cdot (\hat{\Psi} f) = \nabla \hat{\Psi}^\top f + \hat{\Psi} \nabla \cdot f$ .

#### A.4.2 Functional derivative of MF potential functions

Given a functional  $\mathcal{F} : \mathcal{P}(\mathbb{R}^d) \rightarrow \mathbb{R}$  on the space of probability measures, its functional derivative  $F(x, \rho) := \frac{\delta \mathcal{F}(\rho)}{\delta \rho}(x)$  satisfies the following equation

$$\lim_{h \rightarrow 0} \frac{\mathcal{F}(\rho + hw) - \mathcal{F}(\rho)}{h} = \int_{\mathbb{R}^d} F(x, \rho) w(x) dx$$

for any function  $w \in L^2(\mathbb{R}^d)$ . Hence, the derivative of the entropy MF functional  $\mathcal{F}_{\text{entropy}} := \int_{\mathbb{R}^d} \rho(x) \log \rho(x) dx$  can be derived as

$$\begin{aligned} & \lim_{h \rightarrow 0} \frac{1}{h} \left( \mathcal{F}_{\text{entropy}}(\rho + hw) - \mathcal{F}_{\text{entropy}}(\rho) \right) \\ &= \lim_{h \rightarrow 0} \frac{1}{h} \left( \int_{\mathbb{R}^d} \left( hw(x) \log \rho(x) + \rho(x) \frac{hw(x)}{\rho(x)} + \mathcal{O}(h^2) \right) dx \right) \\ &= \int_{\mathbb{R}^d} \left( w(x) \log \rho(x) + w(x) \right) dx = \int_{\mathbb{R}^d} \underbrace{\left( \log \rho(x) + 1 \right)}_{:= F_{\text{entropy}}(x, \rho)} w(x) dx. \end{aligned} \quad (54)$$

Similarly, consider the congestion MF functional  $\mathcal{F}_{\text{congestion}} := \int_{\mathbb{R}^d} \int_{\mathbb{R}^d} \frac{1}{\|x-y\|^2+1} \rho(x) \rho(y) dx dy$ . Its derivation can be computed by

$$\begin{aligned} & \lim_{h \rightarrow 0} \frac{1}{h} \left( \mathcal{F}_{\text{congestion}}(\rho + hw) - \mathcal{F}_{\text{congestion}}(\rho) \right) \\ &= \lim_{h \rightarrow 0} \frac{1}{h} \left( \int_{\mathbb{R}^d} \int_{\mathbb{R}^d} \frac{1}{\|x-y\|^2+1} \left( \rho(x) hw(y) + hw(x) \rho(y) + \mathcal{O}(h^2) \right) dx dy \right) \\ &= \int_{\mathbb{R}^d} \int_{\mathbb{R}^d} \frac{1}{\|x-y\|^2+1} \left( \rho(x) w(y) + w(x) \rho(y) \right) dx dy \\ &= \int_{\mathbb{R}^d} \underbrace{\int_{\mathbb{R}^d} \frac{2}{\|x-y\|^2+1} dy}_{:= F_{\text{congestion}}(x, \rho)} w(x) dx. \end{aligned} \quad (55)$$

We hence conclude the expressions of  $F_{\text{entropy}}$  and  $F_{\text{congestion}}$  in (17).

### A.5 Experiment Details

#### A.5.1 Full setup

**Hyperparameters** Table 6 summarizes the hyperparameters in each MFG, including the dimension  $d$  of the state space, the diffusion scalar  $\sigma$ , the time horizon  $T$ , the discretized time step  $\delta t$  (and  $\delta s$ ), the MF base drift  $f(x, \rho)$ , and finally the MF interaction  $F(x, \rho)$ . Note that in the 1000-dimensional opinion MFG, we multiply the polarized dynamic  $\bar{f}_{\text{polarize}}$  by 6 to ensure that the high-dimensional dynamics yield polarization within the time horizon. Meanwhile, a smaller step size  $\delta t = 0.006$  is adopted so that the discretization error from the relatively large drift is mitigated. As mentioned in Sec. 4, we adopt zero and constant base drift  $f$  respectively for GMM and V-neck/S-tunnel.

Table 6: Expansion of Table 2 to other hyperparameters in each MFG.

|                                           | GMM           | V-neck        | S-tunnel      | Opinion                     |                                     |
|-------------------------------------------|---------------|---------------|---------------|-----------------------------|-------------------------------------|
| $d$                                       | 2             | 2             | 2             | 2                           | 1000                                |
| $\sigma$                                  | 1             | 1             | 1             | 0.1                         | 0.5                                 |
| $T$                                       | 1             | 2             | 3             | 3                           | 3                                   |
| $\delta t$                                | 0.01          | 0.01          | 0.01          | 0.01                        | 0.006                               |
| $f(x, \rho)$                              | $[0, 0]^\top$ | $[6, 0]^\top$ | $[6, 0]^\top$ | $\bar{f}_{\text{polarize}}$ | $6 \cdot \bar{f}_{\text{polarize}}$ |
| diffusion steps                           | 100           | 200           | 300           | 300                         | 500                                 |
| $K^8$                                     | 250           | 250           | 500           | 100                         | 250                                 |
| Number of alternating stages <sup>9</sup> | 40            | 40            | 30            | 40                          | 90                                  |
| Total training steps                      | 20k           | 20k           | 30k           | 8k                          | 45k                                 |

**Boundary distributions** All MFGs adopt Gaussians as their boundary distributions  $\rho_0$  and  $\rho_{\text{target}}$ .

Table 7:  $\rho_0$  and  $\rho_{\text{target}}$  in each MFG. We denote the zero vector and identity matrix respectively by  $\mathbf{0} \in \mathbb{R}^d$  and  $\mathbf{I} \in \mathbb{R}^{d \times d}$ .

| MFG                     | $\rho_0$                                                                                                     | $\rho_{\text{target}}$                                                           |
|-------------------------|--------------------------------------------------------------------------------------------------------------|----------------------------------------------------------------------------------|
| <b>GMM</b>              | $\mathcal{N}(\mathbf{0}, \mathbf{I})$                                                                        | 8 Gaussians, $\mathcal{N}(\mathbf{0}, \mathbf{I})$ , placing at the radius of 16 |
| <b>V-neck</b>           | $\mathcal{N}([-7, 0]^\top, 0.2 \cdot \mathbf{I})$                                                            | $\mathcal{N}([7, 0]^\top, 0.2 \cdot \mathbf{I})$                                 |
| <b>S-tunnel</b>         | $\mathcal{N}([-11, -1]^\top, 0.5 \cdot \mathbf{I})$                                                          | $\mathcal{N}([11, 1]^\top, 0.5 \cdot \mathbf{I})$                                |
| Opinion<br>( $d=2$ )    | $\mathcal{N}(\mathbf{0}, \begin{bmatrix} 0.5 & 0 \\ 0 & 0.25 \end{bmatrix})$                                 | $\mathcal{N}(\mathbf{0}, 3 \cdot \mathbf{I})$                                    |
| Opinion<br>( $d=1000$ ) | $\mathcal{N}(\mathbf{0}, \begin{bmatrix} 4 & & & \\ & 0.25 & & \\ & & \ddots & \\ & & & 0.25 \end{bmatrix})$ | $\mathcal{N}(\mathbf{0}, 3 \cdot \mathbf{I})$                                    |

**Training** All experiments are conducted on 3 TITAN RTXs and 1 TITAN V100 is located on the Amazon Web Service (AWS). We use the multi-step TD targets in (15) for all experiments and adopt huber norm for the TD loss in (16). As for the FK consistency loss  $\mathcal{L}_{\text{FK}}$ , we use  $\ell_1$  norm for GMM and opinion MFGs, and huber norm for the rest.

**Network architecture** All networks  $(Y_\theta, Z_\theta, \hat{Y}_\phi, \hat{Z}_\phi)$  take  $(x, t)$  as inputs and follow

$$\text{out} = \text{out\_mod}(\text{x\_mod}(x) + \text{t\_mod}(\text{timestep\_embedding}(t))),$$

where  $\text{timestep\_embedding}(\cdot)$  is the standard sinusoidal embedding.

For crowd navigation MFGs, these modules consist of 2 to 4 fully-connected layers (Linear) followed by the Sigmoid Linear Unit (SiLU) activation functions [64], *i.e.*,

$$\text{t\_mod} = \text{Linear} \rightarrow \text{SiLU} \rightarrow \text{Linear}$$

$$\text{x\_mod} = \text{Linear} \rightarrow \text{SiLU} \rightarrow \text{Linear} \rightarrow \text{SiLU} \rightarrow \text{Linear} \rightarrow \text{SiLU} \rightarrow \text{Linear}$$

$$\text{out\_mod} = \text{Linear} \rightarrow \text{SiLU} \rightarrow \text{Linear} \rightarrow \text{SiLU} \rightarrow \text{Linear}$$

As for 1000-dimensional opinion MFG, we keep the same  $\text{t\_mod}$  and  $\text{out\_mod}$  but adopt residual networks with 5 residual blocks for  $\text{x\_mod}$ . For DeepGSB-ac, we set the hidden dimension of Linear to 256 and 128 respectively for the policy networks  $(Z_\theta, \hat{Z}_\phi)$  and the critic networks  $(Y_\theta, \hat{Y}_\phi)$ , whereas for DeepGSB-c, we set the hidden dimension of Linear to 200 for the critic networks  $(Y_\theta, \hat{Y}_\phi)$ .

**Implementation of prior methods [14–16]** All of our experiments are implemented with PyTorch [65]. Hence, we re-implement the method in Ruthotto et al. [14] by migrating their Julia codebase<sup>10</sup> to PyTorch. As for the method in Lin et al. [15], their official PyTorch implementation is publicly available.<sup>11</sup> Finally, we implement Chen [16] by ourselves. Since the prior methods [14–16] were developed for a smaller class of MFGs compared to our DeepGSB (recall Table 1), we needed to relax some of the MFG setting adopted in DeepGSB in order for them to yield reasonable results in Fig. 5 and 7. Specifically, we soften the obstacle costs, so that [14, 15] can differentiate them properly, and keep the same KL penalty at  $u(x, T) \approx D_{\text{KL}}(\rho(x, T) || \rho_{\text{target}}(x))$  as adopted in [14, 15]. We stress that neither of the methods [14, 15] works well with the discontinuous  $F_{\text{obstacle}}$  in (17). Finally, we discretize the 2-dimensional state space of GMM into a  $40 \times 40$  grid with 50 time steps for [16]. We note that the complexity of [16] scales as  $\mathcal{O}(\tilde{T}D^2)$ , where  $\tilde{T}$  and  $D$  are respectively the number of time and spatial grids, *i.e.*,  $\tilde{T} = 50$  and  $D = 1600$ .

<sup>7</sup>We note that, unlike SB-FBSDE [27], the number of training iterations at each stage (*i.e.*, the  $K$  in Alg. 1) is kept *fixed* throughout training.

<sup>9</sup>Here, we refer *one alternating stage* to a complete cycling through  $2K$  training iterations in Alg. 1.

<sup>10</sup><https://github.com/EmoryMLIP/MFGnet.jl>. The repository is licensed under MIT License.

<sup>11</sup><https://github.com/atlin23/apac-net>. The repository does not specify licenses.

**Evaluation** We approximate the Wasserstein distance with the Sinkhorn divergence using the geomloss package.<sup>12</sup> The Sinkhorn divergence interpolates between Wasserstein (blur = 0) and kernel (blur =  $\infty$ ) distance given a hyperparameter blur. We set blur = 0.05 in Table 3.

### A.5.2 Additional experiments

Figures 7 and 8 reports the results for **DeepGSB-c**. On crowd navigation MFGs, the population snapshots guided by DeepGSB-c are visually indistinguishable from DeepGSB-ac (see Fig. 7 vs. 5) despite the visual difference in their contours. As for 1000-dimensional opinion MFG, both DeepGSB-c and DeepGSB-ac are able to guide the population opinions toward desired  $\rho_{\text{target}}$  without the entropy interaction  $F_{\text{entropy}}$ . Figure 8 reports the results of DeepGSB-c in such cases. We note, however, that when  $F_{\text{entropy}}$  is enabled, DeepGSB-ac typically performs better than DeepGSB-c in terms of convergence to  $\rho_{\text{target}}$  and training stability.

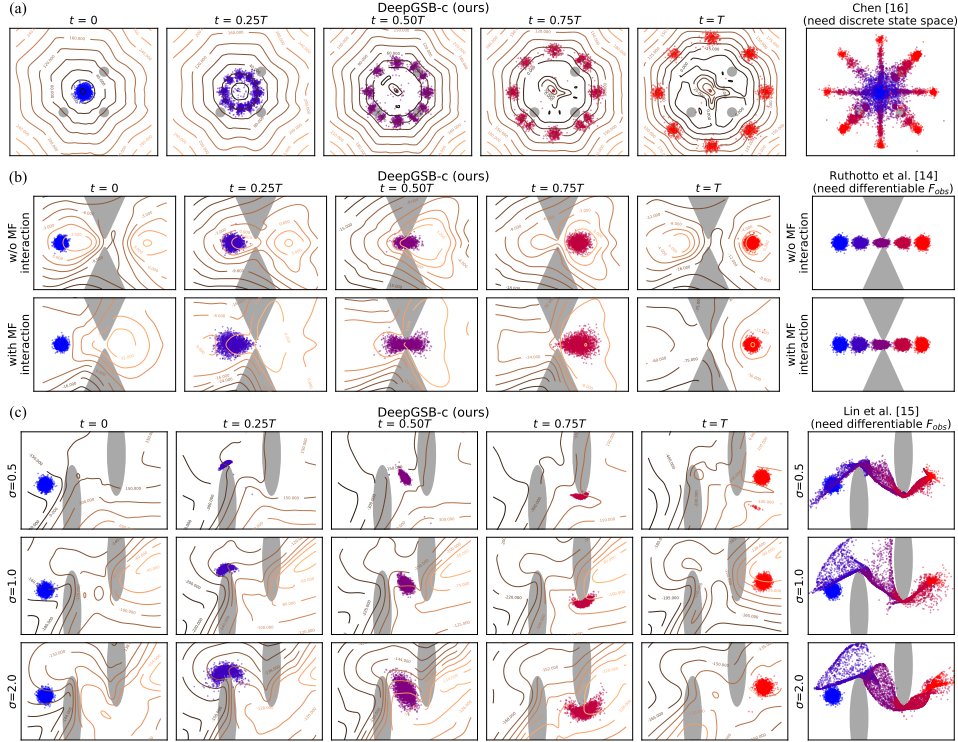

Figure 7: Same setup as in Fig. 5 except for **DeepGSB-c**. This figure is best viewed in color.

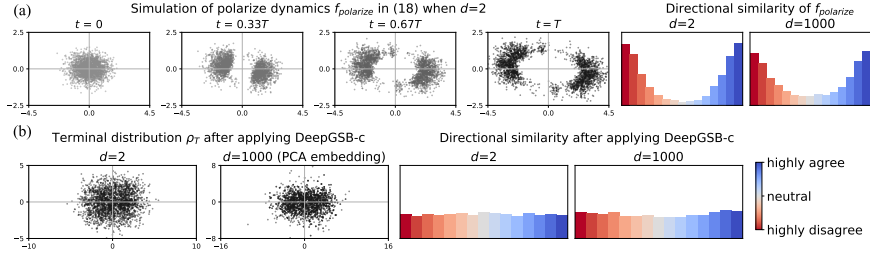

Figure 8: (a) Visualization of polarized dynamics  $\bar{f}_{\text{polarize}}$  in 2- and 1000-dimensional opinion space, where the *directional similarity* [3] counts the histogram of cosine angle between pairwise opinions at the terminal distribution  $\rho_T$ . (b) **DeepGSB-c** guides  $\rho_T$  to approach moderated distributions, hence *depolarizes* the opinion dynamics. Note that we adopt  $F := 0$  for DeepGSB-c. We use the first two principal components to visualize  $d=1000$ .

<sup>12</sup><https://github.com/jeanfeydy/geomloss>. The repository is licensed under MIT License.

## A.6 Additional Clarifications (for Rebuttal)

### A.6.1 Additional remarks

**Solvability of general IPF & Sinkhorn to (7).** It is known that the PDE proposed in (7) admits a variational optimization form [32]:

$$\begin{aligned} & \min_{\rho, u} \int_{\mathbb{R}^d} \int_t \left( \frac{1}{2} \|u(x, t)\|^2 + \mathcal{F}(\rho(x, t)) \right) \rho(x, t) dt dx, \\ \text{s.t. } & \frac{\partial \rho(x, t)}{\partial t} - \nabla \cdot (\rho (\sigma^2 \nabla u - f)) - \frac{1}{2} \sigma^2 \Delta \rho = 0, \\ & \rho(x, 0) = \rho_0(x), \quad \rho(x, T) = \rho_{\text{target}}(x), \end{aligned}$$

where  $\mathcal{F}$  relates to  $F$  via functional derivative (see Appendix A.4.2 and Ruthotto et al. [14]). This stochastic optimal control problem, after discretization, yields

$$\min_{M \in \Pi(\rho_0, \rho_{\text{target}})} \langle C(M), M \rangle + \langle \log M, M \rangle \quad (56)$$

where  $M$  is a  $(T + 1)$ -dimensional tensor with  $M(x_0, \dots, x_T)$  representing the probability of  $P(X_0 = x_0, \dots, X_T = x_T)$ , and  $C(M)$  is the cost tensor. When the mean-field uncontrolled base drift is independent of population density,  $f := f(x)$ , and mean-field preference  $\mathcal{F}(\rho)$  is convex in  $\rho$ , the optimization in (56) admits convex structure; hence general IPF and Sinkhorn enjoy global convergence. This is essentially what has been proposed in Chen [16], which we detailed in Table 1 and compared extensively with our DeepGSB in Fig. 5. We note that for generic mean-field dynamics, such as the polarized  $f(x, \rho)$  in our (18), the problem (56) is in general non-convex; hence only local convergence can be established (see Remark 1 in [16]).

**Remarks on convergence & relation of Alg. (1) to TRPO [51].** The alternating optimization scheme proposed in Alg. (1) can be compactly presented as  $\min_{\phi} D_{\text{KL}}(q^{\theta} || q^{\phi}) + \mathbb{E}_{q^{\theta}}[\mathcal{L}_{\text{TD}}(\phi)]$  and  $\min_{\theta} D_{\text{KL}}(q^{\phi} | q^{\theta}) + \mathbb{E}_{q^{\phi}}[\mathcal{L}_{\text{TD}}(\theta)]$ . Despite that the procedure seems to resemble IPF, which optimizes between  $\min_{\phi} D_{\text{KL}}(q^{\phi} | q^{\theta})$  and  $\min_{\theta} D_{\text{KL}}(q^{\theta} | q^{\phi})$ , we stress that they differ from each other in that the KLs are constructed with different directions.

In cases where the TD objectives are discarded, prior work [24] has proven that minimizing the forward KLs admit similar convergence to standard IPF (which minimizes the reversed KLs). This is essentially the key to developing scalable methods, since the parameter being optimized (e.g.,  $\theta$ ) in forward KLs differs from the parameter used to sample expectation (e.g.,  $\mathbb{E}_{q^{\phi}}$ ). Therefore, the computational graph of the SDEs can be dropped, yielding a computationally much efficient framework. These advantages have been adopted in [24, 27] and also this work for solving higher-dimensional problems.

However, when we need TD objectives to enforce the MF structure, as appeared in all the MFGs in this work, the combined objective does not correspond to IPF straightforwardly. Despite that the alternating procedure in Alg. (1) is mainly inspired by prior SB methods [24, 27], the training process of DeepGSB is perhaps closer to TRPO [51], which iteratively updates the policy using the off-policy samples generated from the previous stage:  $\pi^{(i+1)} = \arg \min_{\pi} D_{\text{KL}}(\pi^{(i)} || \pi) + \mathbb{E}_{\pi^{(i)}}[\mathcal{L}(\pi)]$ . TRPO is proven to enjoy monotonic improvement over iterations (i.e., local convergence). For general MFGs where the uncontrolled dynamic  $f := f(x, \rho)$  depends on population density  $\rho$ , both methods (DeepGSB and e.g., Chen [16]) admit local convergence. When the MFG is simplified (like GMM) such that its discrete problem admits convex structure, we still observe empirically that DeepGSB converges smoothly (see Fig. 10), whereas the reconstructed policy from Chen [16] can suffer from discretization errors.

**Additional discussion on Diffusion Schrödinger Bridge (DSB) [24].** For completeness, we note that DSB [24] is an independently developed numerical SB solver closely related to SB-FBSDE [27]. The two methods had been shown to share the *same* IPF objectives, e.g.,  $\mathbb{E}[\|Z_{\theta} + \hat{Z}_{\phi} - \sigma \nabla \log q^{\theta}\|^2]$ , except adopting different approximation techniques. Specifically, while SB-FBSDE replaces the intractable  $\nabla \log q^{\theta}$  with the divergence using integration by parts (see Lemma 5), DSB instead performs  $\mathbb{E}[\|Z_{\theta} + \hat{Z}_{\phi} - \sigma \nabla \log q^{\theta}\|^2] \propto \mathbb{E}[\|Z_{\theta} + \hat{Z}_{\phi} - \sigma \nabla \log q^{\theta}(X_k | X_{k-1})\|^2]$ , then estimates  $\nabla \log q^{\theta}(X_k^{\theta} | X_{k-1}^{\theta})$  with forward samples  $(X_{k-1}^{\theta}, X_k^{\theta}, Z_{\theta})$  (as it is a tractable Gaussian kernel). We refer readers of interest to Appendix C in [27] for more details.

Since the objective in SB-FBSDE is equivalent to the one in DSB, issues arising in SB-FBSDE will also be faced in DSB. Hence, while DSB indeed provides a simpler regression objective compared to SB-FBSDE, both methods are insufficient to solve the MFG PDE in (7). Specifically, they will converge to the entropy-regularized OT solution with degenerate MF structure  $F := 0$ . In this vein, by first decomposing the MFG PDE (7) into its equivalent FBSDEs (11,12), then recognizing the underlying TD structure, additional objectives can be introduced to encourage training to respect nontrivial  $F$ . Further, it naturally handles non-differentiable  $F$ , which offers extra benefits in many cases. We highlight it as a distinct benefit from FBSDE methods, that is otherwise absent in [24].

However, we also note that the divergences appearing in FBSDE-based objectives may scale unfavorably as the dimension grows, as they are often approximated by the Hutchinson trace estimator [66], which exhibits high variance in higher dimension. This limitation may be mitigated by replacing them with the simpler (yet equivalent) regression objectives used in DSB, which enjoy lower variance.

### A.6.2 Additional experiments

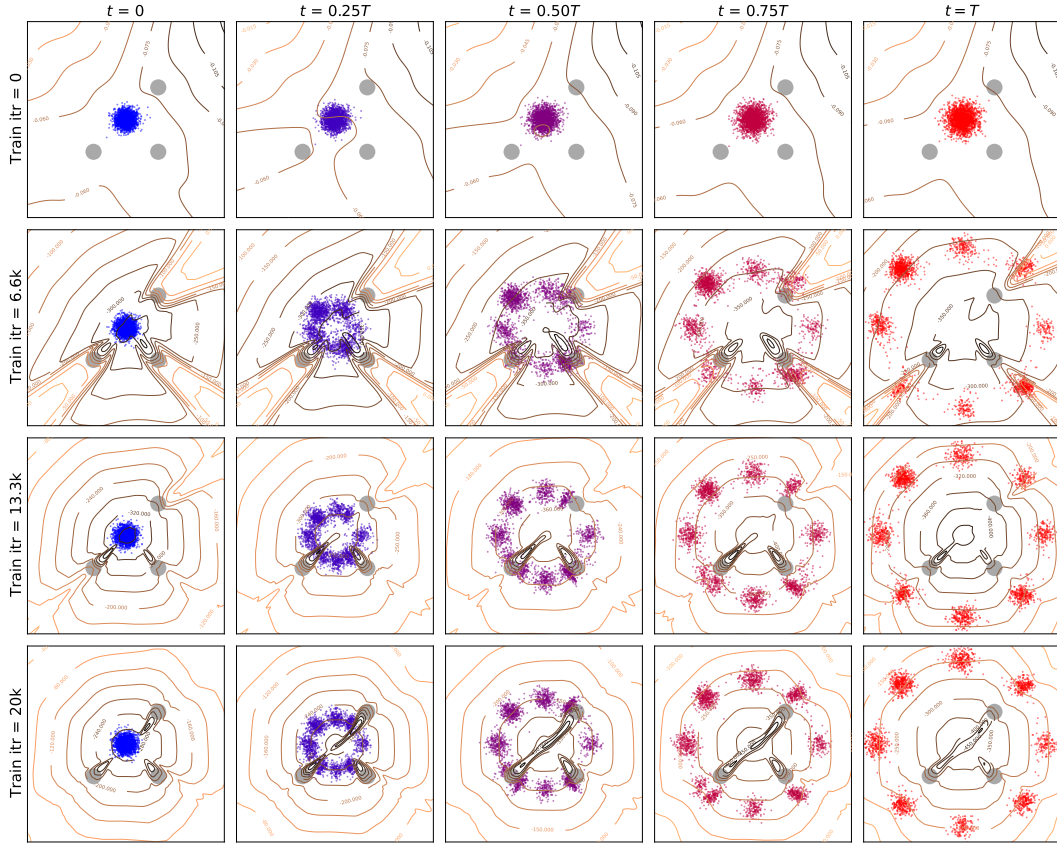

Figure 9: Visualization of DeepGSB-ac training on **GMM**, where each row represents a policy snapshot at different training stages, from initialization (top row) to convergence (bottom row).



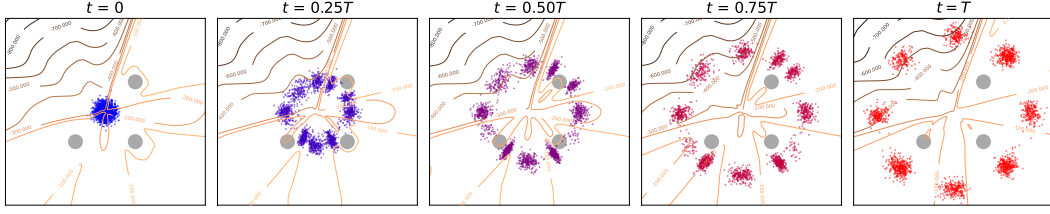

Figure 10: Results of DeepGSB-ac on **GMM** when trained *without*  $\text{TD}_0$  and  $\widehat{\text{TD}}_0$ . In other words, the training process does not requires knowing  $\rho_0$  and  $\rho_{\text{target}}$ , but only samples from  $X_0 \sim \rho_0$  and  $\bar{X}_0 \sim \rho_{\text{target}}$ . Notice that the contour of  $Y_\theta$  differs from Fig. 5, yet the policy is able to generate similar trajectories.

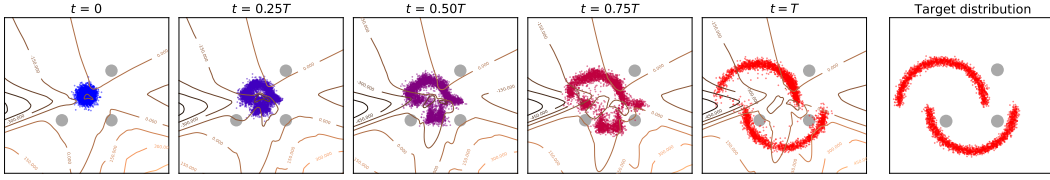

Figure 11: Results of DeepGSB-ac when trained *without*  $\text{TD}_0$  and  $\widehat{\text{TD}}_0$ , with a unknown target distribution. The training process does not requires knowing  $\rho_0$  and  $\rho_{\text{target}}$ , but only samples from  $X_0 \sim \rho_0$  and  $\bar{X}_0 \sim \rho_{\text{target}}$ .
